# Supplementary material for: On-the-fly machine learning force field generation: Application to melting points
Source: arXiv:1904.12961 ancillary file (2019-05-05)
Supplement: Supplementary file 1 [file Supplementary_Materials_Jinnouchi.pdf]

**Supplemental Material**

# On-the-fly machine learning force field generation:

# Application to melting points

Ryosuke Jinnouchi,[1,2] Ferenc Karsai,[3] and Georg Kresse[1,3]

1. University of Vienna, Department of Physics, Sensengasse 8, Vienna, Austria
2. Toyota Central R&D Labs., Inc., 41-1 Yokomichi, Nagakute, Aichi 480-1192, Japan
3. VASP Software GmbH, Sensengasse 8, Vienna, Austria

**Contents**

**S1 Parameters in descriptor and kernel**

**S2 Parameters and models used in MD training simulations**

**S3 Computational efficiency**

**S4 Parameters and models for interface pinning calculations**

## S1 Parameters in descriptor and kernel

The parameters listed in Table S1 were used for the descriptors and kernel for all materials.

**Table S1** Parameters for descriptor and kernel

| Parameter | Value | Parameter | Value |
|---|---|---|---|
| $\sigma_{atom}$ | 0.5 Å | $L_{max}$ | 6 |
| $R_{cut}$ for angular descriptor | 5 Å | $\zeta^{(3)}$ | 4 |
| $\beta^{(2)}$ | 0.0 | $N^{l}_{R}$ for angular | 9 ($l$=0), 8 ($l$=1 and 2), 7 ($l$=3 and 4) and 6 ($l$=5 and 6) |
| $\beta^{(3)}$ | 1.0 | Spline mesh | 100 |

## S2 Parameters and models used in MD training simulations

The simulation conditions and models used for the on-the-fly force field generations are summarized in Table S2 and Fig. S1. In this study, all MD simulations for the force field generations were executed under the NVT ensemble with a Langevin thermostat [48]. However, it should be noted that there is no obstacle in using the NPT ensemble in our developed on-the-fly force-field generation program as shown in Ref. [23].

The initial structures of these MD simulations were prepared as follows. In advance of the MD simulations on solids at 300 K, structures at 0 K were obtained by using first principles calculations, and the optimized structures were equilibrated by MD simulations for 20 ps under the NPT ensemble at 300 K and 0.1 MPa. In these equilibration simulations, we also adopted the on-the-fly scheme, where many steps of the MD simulations were replaced by the evolved force fields, in order to accelerate the structural preparations. Equilibrium lattice constants were determined by these equilibrations, and the structures at 0 K obtained by the first principles calculations were adjusted to the determined equilibrium lattice constants. These adjusted structures were used as the initial structures of the MD simulations under the NVT ensemble at 300 K for the force field generations. The equilibrium lattice constants at higher temperatures were determined by the same method. The final structures provided by the simulations at 300 K were adjusted to these lattice constants and used as the initial structures of the force field generations.

The liquid structures were prepared by melting the Al, Si, Ge, Sn and MgO solids for 100 ps by MD simulations under the $NP_zT$ ensemble at 2000 K, 3000 K, 2000 K,

1000 K and 5000 K, respectively, by using the on-the-fly molecular dynamics scheme. In these $NP_zT$ ensemble simulations, the lattice constant along the *z*-axis was controlled to provide the ambient pressure, whereas the lattice constants within the *xy*-plane were fixed at those of solids determined by the high-temperature simulations. After the melting, the systems were equilibrated for 20 ps at the target temperatures, and the equilibrium lattice constant along the *z*-axis was determined. Then, the final liquid structures were adjusted to the equilibrium lattice constant and used as the initial structures of the MD simulations under the NVT ensemble for the force field generations.

Preparations for the initial interfacial structures are similar to those for the liquids. Differences are only in their melting simulations, where only a half of the atoms in each system were relaxed from their initial solid positions, and simulations were executed under the NVT ensemble. In the NVT ensemble simulations on the interfaces, the small interfacial systems sometimes melted (or crystalized) to pure liquid (or solid) when the simulation temperatures were set to be far from the melting points. Thus, estimations of the melting points are necessary to properly collect the reference configurations of interfaces. Because of this reason, we estimated in advance of the training on the interfaces the temperatures, where the interfaces are stable. This is achieved by using a bisection method. Within this method, we only used force fields generated from the reference datasets on solids and liquids. Furthermore, in order to stabilize the interfaces, we applied harmonic bias potentials during the MD simulations as in the interface pinning calculations.

**Table S2** Simulation conditions for training of machine-learning force fields.

| | System | Simulation condition |
|---|---|---|
| Al | $Al_{108}$ solid (fcc) | 300 and 1000 K under NVT ensemble. |
| | $Al_{108}$ liquid | 2000 K under NVT ensemble. |
| | $Al_{144}$ interface | 900 K for LDA, 850 K for PBE, and 1000 K for PBEsol and SCAN under NVT ensemble with a harmonic bias potential adopted in the interface pinning method. |
| Si | $Si_{64}$ solid ($\alpha$-tin) | 300 and 1500 K under NVT ensemble. |
| | $Si_{64}$ liquid | 2000 K under NVT-ensemble. |
| | $Si_{128}$ interface | 1300 K for LDA, PBE and PBEsol and 1800 K for SCAN under NVT ensemble with a harmonic bias potential adopted in the interface pinning method. |
| Ge | $Ge_{64}$ solid ($\alpha$-tin) | 300 and 1300 K under NVT ensemble. |
| | $Ge_{64}$ liquid | 2000 K under NVT ensemble. |
| | $Ge_{128}$ interface | 800 K for LDA, 900 K for PBE, 950 K for PBEsol and 1200 K for SCAN under NVT ensemble with a harmonic bias potential adopted in the interface pinning method. |
| Sn | $Sn_{64}$ solid ($\beta$-tin) | 300, 400 and 500 K under NVT ensemble. |
| | $Sn_{64}$ liquid | 1000 K under NVT ensemble. |
| | $Sn_{128}$ interface | 500 K under NVT ensemble with a harmonic bias potential adopted in the interface pinning method. |
| MgO | $(MgO)_{32}$ solid (rock salt) | 300 and 3000 K under NVT ensemble. |
| | $(MgO)_{32}$ liquid | 4000 K under NVT ensemble. |
| | $(MgO)_{64}$ interface | 3400 K for LDA, 3100 K for PBE, 3300 K for PBEsol and 3400 K for SCAN under NVT ensemble with a harmonic bias potential adopted in the interface pinning method. |

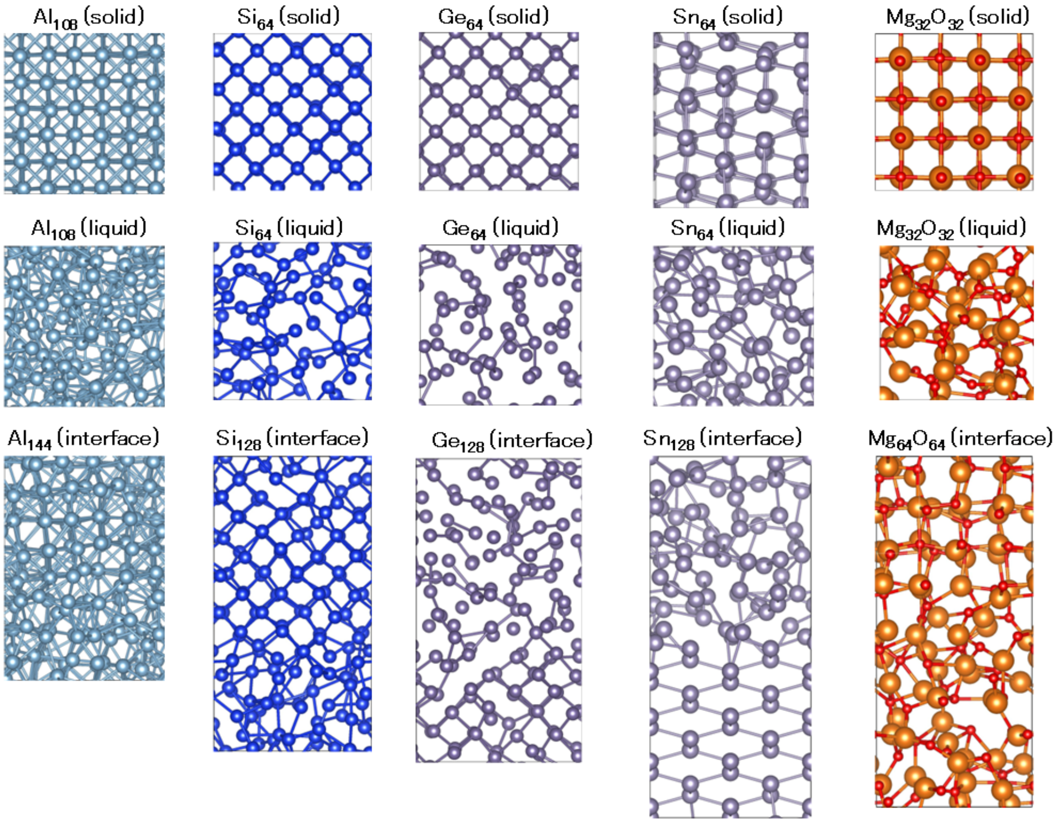


**Figure S1** Solid, liquid and interface models of Al, Si, Ge, Sn and MgO used in on-the-fly force field generations.

## S3 Computational efficiency

The data showing the computational efficiency of the on-the-fly force field generations is tabulated in Table S3, the number of structures providing the reference structure datasets and the number of the local reference configurations are tabulated in Table S4, and the elapsed time per MD step by the generated force fields are summarized in Table S5.

**Table S3** Fraction $x_1$ (%) of the MD steps, where FP calculations were bypassed, and acceleration factor $x_2$ of the 100 ps MD simulation by the on-the-fly scheme using the SCAN functional.

| | State | $x_1$ | $x_2$ | | State | $x_1$ | $x_2$ |
|---|---|---|---|---|---|---|---|
| Al | Solid (300 K) | 99.9 | 942 | Sn | Solid (300 K) | 99.6 | 220 |
| | Solid (1000 K) | 99.7 | 290 | | Solid (400 K) | 99.6 | 217 |
| | liquid (2000 K) | 99.6 | 264 | | Solid (500 K) | 98.0 | 48 |
| | Interface (1000 K) | 99.4 | 158 | | Liquid (1000 K) | 98.9 | 89 |
| | | | | | Interface (500 K) | 99.9 | 867 |
| Si | Solid (300 K) | 99.6 | 263 | MgO | Solid (300 K) | 99.8 | 435 |
| | Solid (1500 K) | 99.7 | 364 | | Solid (3000 K) | 99.6 | 251 |
| | liquid (2000 K) | 99.4 | 170 | | Liquid (4000 K) | 99.1 | 114 |
| | Interface (1800 K) | 99.6 | 253 | | Interface (3000 K) | 99.7 | 275 |
| Ge | Solid (300 K) | 99.9 | 1569 | Ge | liquid (2000 K) | 99.6 | 239 |
| | Solid (1300 K) | 99.7 | 364 | | Interface (1800 K) | 99.3 | 150 |

**Table S4** The number $N_{st}$ of structures providing the reference structure datasets and the number $N_B$ of local reference configurations.

| | XC | State | $N_{st}$ | $N_B$ | | XC | State | $N_{st}$ | $N_B$ |
|---|---|---|---|---|---|---|---|---|---|
| Al | LDA | Solid | 79 | 128 | Si | LDA | Solid | 179 | 390 |
| | | liquid | 140 | 530 | | | Liquid | 79 | 344 |
| | | interface | 35 | 37 | | | Interface | 74 | 82 |
| | PBE | Solid | 90 | 142 | | PBE | Solid | 140 | 398 |
| | | liquid | 139 | 525 | | | Liquid | 171 | 517 |
| | | interface | 57 | 57 | | | Interface | 83 | 83 |
| | PBEsol | Solid | 56 | 146 | | PBEsol | Solid | 86 | 419 |
| | | liquid | 282 | 712 | | | Liquid | 139 | 400 |
| | | interface | 5 | 5 | | | Interface | 72 | 73 |
| | SCAN | Solid | 108 | 206 | | SCAN | Solid | 117 | 154 |
| | | liquid | 124 | 508 | | | Liquid | 193 | 538 |
| | | interface | 49 | 51 | | | Interface | 88 | 91 |
| Ge | LDA | Solid | 159 | 249 | MgO | LDA | Solid | 207 | 387 (Mg), 312 (O) |
| | | liquid | 123 | 313 | | | Liquid | 652 | 708 (Mg), 909 (O) |
| | | interface | 79 | 118 | | | Interface | 156 | 63 (Mg), 119 (O) |
| | PBE | Solid | 171 | 287 | | PBE | Solid | 192 | 345 (Mg), 345 (O) |
| | | liquid | 163 | 284 | | | Liquid | 624 | 842 (Mg), 1072 (O) |
| | | interface | 103 | 109 | | | Interface | 81 | 87 (Mg), 74 (O) |
| | PBEsol | Solid | 130 | 229 | | PBEsol | Solid | 139 | 338 (Mg), 286 (O) |
| | | liquid | 81 | 342 | | | Liquid | 690 | 730 (Mg), 928 (O) |
| | | interface | 101 | 109 | | | Interface | 154 | 100 (Mg), 126 (O) |
| | SCAN | Solid | 86 | 518 | | SCAN | Solid | 152 | 289 (Mg), 278 (O) |
| | | liquid | 135 | 359 | | | Liquid | 283 | 454 (Mg), 588 (O) |
| | | interface | 41 | 42 | | | Interface | 115 | 108 (Mg), 174 (O) |
| Sn | SCAN | Solid | 110 | 470 | | | | | |
| | | Liquid | 279 | 324 | | | | | |
| | | Interface | 9 | 207 | | | | | |

**Table S5** Elapsed time (s) per MD step for the interfaces shown in Fig. S2 by the MLFF and FP method. The SCAN functional on a single **k**-point (Γ-point ) was employed in all DFT calculations. Other parameters are the same as those described in Section E. All test calculations were executed by using 48 Intel® XEON® E5-2650 (v2) 2.60 GHz cores.

| | DFT | MLFF | | DFT | MLFF |
|---|---|---|---|---|---|
| $Al_{512}$ | 455 | 0.14 | $Sn_{672}$ | 406 | 0.18 |
| $Si_{672}$ | 954 | 0.19 | $(MgO)_{216}$ | 1621 | 0.50 |
| $Ge_{672}$ | 516 | 0.20 | | | |

## S4 Parameters and models for interface pinning calculations

Figure S2 shows the models used in the interface pinning calculations. As the order parameter, we adopted the collective density $Q = |\rho_{\mathbf{q}}|$, where $\rho_{\mathbf{q}}=1/N^{-1/2}\Sigma_j \exp(-i\mathbf{q}\cdot\mathbf{r}_j)$, $\mathbf{q}=(f_1\mathbf{b}_1,f_2\mathbf{b}_2,f_3\mathbf{b}_3)$, and $\mathbf{b}_k$ is the reciprocal primitive vector. The parameters $f_k$ were determined to maximize the difference in the order parameter between the solid and liquid. The determined parameters are tabulated in Table S6. A 100 ps MD simulation using the NPT ensemble was executed on both solid and liquid to obtain the averages of the order parameter $<Q>$ and enthalpy, and a 200 ps MD simulation under the $NP_zT$ ensemble was executed on each interface to obtain the average of the order parameter $<Q>'$. By using these averages and the thermodynamic relationship, $\partial\Delta\mu/\partial T|_p = -\Delta s = -(\Delta H-\Delta\mu)/T$, the necessary temperature change to satisfy $\Delta\mu = 0$ was estimated as $\Delta\mu/\Delta s$ by using a Newton's method for root finding. This procedure was iteratively executed until the temperature converged within 10 K. The final $\Delta\mu/\Delta s$ and the uncertainty determined by a block averaging method were used to determine the error bar in the melting point. In all MD simulations, the temperature was controlled by the Langevin thermostat [48], and the pressure was controlled by the Parrinello-Rahman method [56, 57]. Time steps were set as 3fs for Al, Si, 10 fs for Ge and Sn, and 2 fs for MgO.

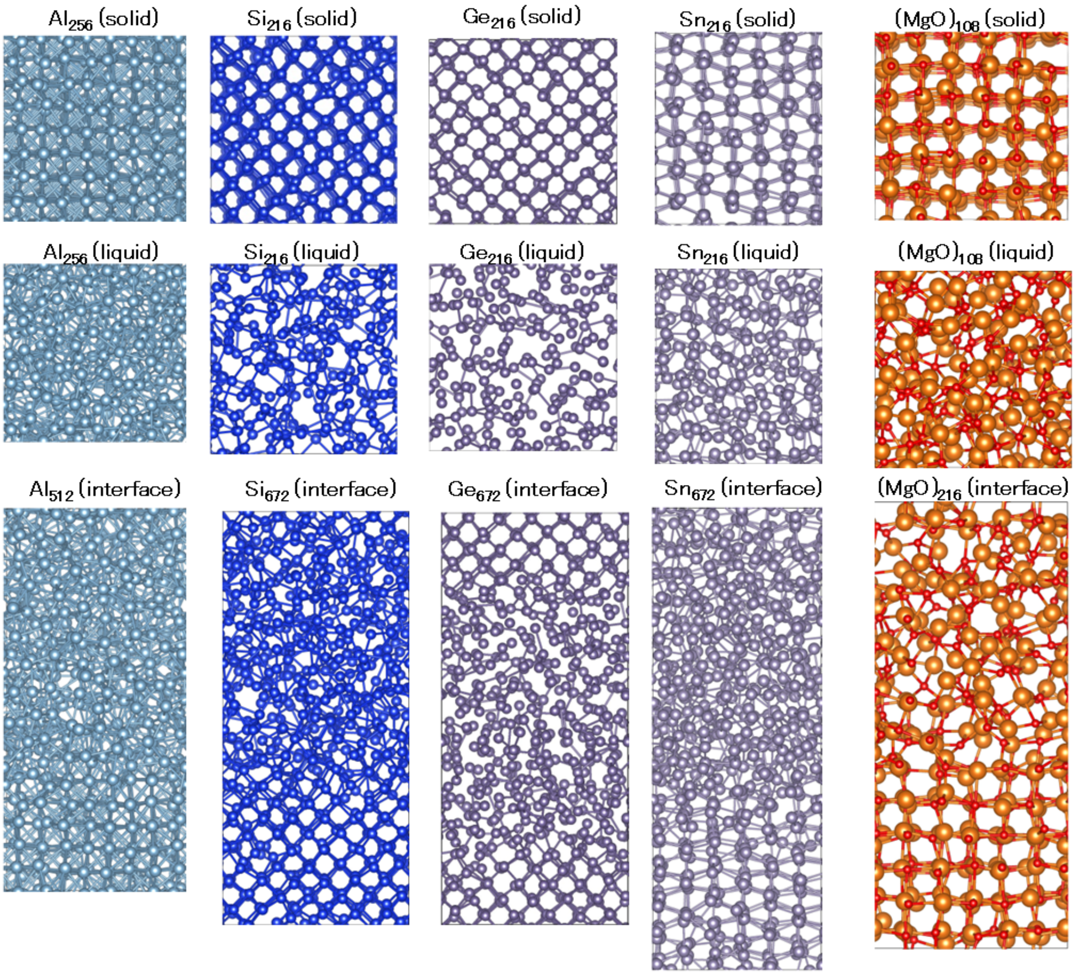


**Figure S2** Solid, liquid and interface models used in the interface pinning calculations.

**Table S6** Order parameters ($f_1$,$f_2$,$f_3$), force constant $\kappa$ (eV) and target order parameter $a$ used in the interface pinning calculations. The target value was set as an average of order parameters of solid and liquid.

| . | ($f_1$, $f_2$, $f_3$) | Force constant, $\kappa$ | Target value $a$ |
|---|---|---|---|
| Al | (8, 0, 0) | 10 | 7.0 |
| Si | (12, 0, 0) | 10 | 5.6 |
| Ge | (12, 0, 0) | 10 | 5.6 |
| Sn | (12, 0, 0) | 10 | 7.0 |
| MgO | (5.84, 0, 0) | 10 | 9.0 |
